# Supplementary material for: Consistent Robust Adversarial Prediction for General Multiclass Classification
Source: arXiv:1812.07526 source file (2019-11-20)
Supplement: Supplementary file 1 [file appendix.tex]

\appendix

\allowdisplaybreaks

\section{Proofs for Section 3}

\subsection{Proof for Theorem 4}

    The $\text{AL}^{\text{0-1}}$ above corresponds to the set of extreme points where the non-zero elements of $\qvec$ (we denote the set containing this elements as $S$) has uniform probability of $\frac{1}{|S|}$ and the value of $v$ is $\frac{|S|-1}{|S|}$. 
    Denote the convex polytope defined by the convex hull of this set of extreme points as $\Dbb$. We need to show that $\Dbb$ is equal to the convex polytope $\Cbb$ formed by the constraints in Eq. \eqref{eq:al-lp} when $\Lbf$ is the zero-one loss matrix. 

    First, we prove that $\Dbb \subseteq \Cbb$ by showing that every extreme point in $\Dbb$ is also an extreme point in $\Cbb$.
    For the case of the multiclass zero-one loss metric, the rank of $\Abf$ (the coefficient matrix in Eq. \eqref{eq:polytope-half-space}) is $k + 1$ (full column rank). 
    For each extreme point $\begin{bmatrix} \qvec \\ v \end{bmatrix}$ in $\Dbb$ where $S$ is the non-zero component of $\qvec$, we construct the corresponding equality subsystem of the polytope $\Cbb$ by selecting all $i$-th rows where $i \in S$ of the first block of $\bf A$, and all $j$-th rows where $j \not\in S$ of the second block, as well as the sum-to-one equality from the third block resulting in $k+1$ linearly independent rows of $\bar{\Abf}$.
    Let $\bar{\qvec}, \bar{v}$ be the solution of this equality subsystem. Satisfying the selected equalities from the first block means that all $\bar{q}_i, \forall i \in S$ need to have the same value. The selected equalities from the second block require that $\bar{q}_j = 0, \forall j \not\in S$. Finally, the sum-to-one equality enforces $\bar{q}_i = \frac{1}{|S|}, \forall i \in S$. Any of the selected equalities from the first block enforces $\bar{v} = \frac{|S|-1}{|S|}$. Therefore, the solution for this equality subsystem is exactly the same as the extreme point in $\Dbb$ we started with, which implies $\Dbb \subseteq \Cbb$.
    
    To complete our proof that $\Dbb = \Cbb$, we need to show that there are no additional extreme points in $\Cbb$. We will show that any equality subsystem with $\rank(\bar{A}) = k+1$ in $\Cbb$ will not produce additional extreme points. 
    We now consider the case where the selected rows form the first block and second block have overlaps rather than mutual exclusivity as in our previous construction. Since there are overlaps, the equalities require that $\bar{q}_i = 0$ for all $i$ in the selected indices from the first and second block. 
    If there is only one index $j$ left unselected, then the solution is to set $q_j = 1$ and 0 for the rest, which we already considered in the previous extreme points construction.
    Otherwise, if they are more than one, then $\rank(\bar{A})$ will be less than $k+1$ since since columns of $\bar{A}$ corresponding to the unselected indices have the same value. 
    The last case is when we select all $k$ rows from the second block. In this case, $\rank(\bar{A}) < k + 1$ since the third block is linearly dependent with all $k$ rows from the second block.
    In conclusion, we show that there are no additional extreme points in $\Cbb$, and hence $\Dbb = \Cbb$. Thus, maximizing over the set of extreme points in $\Dbb$ results in the definition of $\text{AL}^{\text{0-1}}$ above.

\subsection{Proof for Theorem 5}

    The $\text{AL}^{\text{ord}}$ above corresponds to the set of extreme points where only one or two non-zero elements of $\qvec$ are possible
    (note that $i$ and $j$ can have the same value) with uniform probability of $\frac{1}{2}$ and the value of $v$ is $\frac{j-i}{2}$. 
    Let us call the convex polytope defined by the convex hull of this set of extreme points as $\Dbb$. We need to show that $\Dbb = \Cbb$. 

    Our proof technique is similar with the case of zero-one loss metric. 
    First, we show that every extreme point in $\Dbb$ is also an extreme point in $\Cbb$.
    For each extreme point in $\Dbb$ with two non-zero components of $\qvec$ (let us call it $i$ and $j$), we construct the corresponding equality subsystem of the polytope $\Cbb$ by selecting all $i$-th and $j$-th rows from the first block of $\bf A$ (only select one row if $i = j$), and the remaining indices from the second block, with the  sum-to-one equality resulting in $k+1$ linearly independent rows of $\bar{\Abf}$.
    Let $\bar{\qvec}, \bar{v}$ be the solution of this equality subsystem. Satisfying the selected equalities from the second block means all elements of $\bar{\qvec}$ have zero values except $i$-th and $j$-th elements. The selected equalities from the first block combined with the sum-to-one constraint require that $\bar{q}_i = \bar{q}_j = \frac12$. The $i$-th and $j$-th equalities from the first block enforces $\bar{v} = \frac{j-i}{2}$. The solution for this equality subsystem is exactly the same as the extreme point in $\Dbb$ we started with.
    
    To complete our proof that $\Dbb = \Cbb$, w will show that any equality subsystem with $\rank(\bar{A}) = k+1$ in $\Cbb$ will not produce additional extreme points. There are few cases that we need to have a look:
    \begin{enumerate}%[noitemsep,topsep=0pt]
        \item The indices selected from the first block and second block are mutually exclusive. \\
        Let $i$ and $j$ be the minimum and the maximum indices from the selected rows of the first block respectively.
        The solution of this equality subsystem is to set $\bar{q}_i = \bar{q}_j = \frac12$ and $\bar{v} = \frac{j-i}{2}$, while setting the other indices of $\bar{\qvec}$ as 0 despite being selected from the first block. By setting the value of $\bar{\qvec}$ and $\bar{v}$ as above, it automatically satisfies any $l$-th equation in the first block where $i\leq l \leq j$ since the coefficient of $i$-th and $j$-th columns of $l$-th row of the loss matrix sum to $j-i$.
        The resulting extreme point in this case is already in our consideration.
        \item The indices selected from the first block overlap with the ones from the second block.\\
        Since selecting $i$-th row of the second block means assigning 0 probability to $\bar{q}_i$, we can define an equivalent equality with the resulting equality subsystem by taking the rows from the first block as well as the sum-to-one constraint, and removing the columns correspond to the selected rows from the second block. Let us call the set of selected rows from the first block as $S$ and the set of remaining column indices as $R$. The are two different cases:
        \begin{enumerate}[label=\alph*] %.,noitemsep,topsep=0pt]
            \item The case where $\min(R) \le \min(S)$, and $\max(R) \ge \max(S)$. \\
            If $\rank(\bar{A}) = k+1$, then the solution for equality subsytem in this case is to set $\bar{q}_{\min(R)} = \bar{q}_{\max(R)} = \frac12$ and 0 for the rest, with $\bar{v} = \frac{\max(R) - \min(R)}{2}$. Similar to the first case, this will automatically satisfies any $l$-th equation in the first block where $\min(R)\leq l \leq \max(R)$.  The resulting extreme point is also already in our consideration.
            \item The case where $\min(S) < \min(R)$, or $\max(S) > \max(R)$. \\
            In this case, satisfying the $i$-th equality from the first block where $i < \min(R)$ or $i > \max(R)$ and the non-negative constraints will make the value of $\bar{v}$ big such that the $j$-th inequality where $\min(R) \le j \le \max(R)$ cannot be satisfied since $\Lbf_{(j,:)} \qvec < \bar{v}$. This makes the solution of the system of equation lies outside the polytope $\Cbb$, and hence, it is not an extreme point of $\Cbb$.
        \end{enumerate}
    \end{enumerate}

    Therefore, we show that there is no additional extreme points in $\Cbb$, and hence $\Dbb = \Cbb$, which concludes our proof.

\subsection{Proof for Theorem 6}

    The $\text{AL}^{\text{sq}}$ above corresponds to the set of extreme points where only a single element of $\qvec$ is non zero with probability of one, or two non-zero elements of $\qvec$ are allowed 
    (let us call them $i$ and $j$) where the probability of $q_i = \frac{ 2(j - l) + 1}{2 \left(j - i \right)}$ and $q_j = \frac{ 2(l - i) - 1}{2 \left(j - i \right)}$ for any $i,j,l \in \{1,\hdots,k\}, i < l \leq j $ with the value of $v$ is $\frac{ \left( 2(j - l) + 1 \right) \left( l \!-\! i \right)^2  +
	  \left( 2(l \!-\! i) \!-\! 1 \right) \left( j \!-\! l \right)^2 }
	  {2 \left(j - i \right)}$. 
    Let us call the convex polytope defined by the convex hull of this set of extreme points as $\Dbb$. We need to show that $\Dbb = \Cbb$. 

    First, we show that every extreme point in $\Dbb$ is also an extreme point in $\Cbb$.
    We note that each row in the first block of the coefficient matrix $\Abf$ in Eq. \eqref{eq:polytope-half-space} can be written as a linear combination of two other rows in the first block and the sum-to-one row in the third block. This follows the corresponding relation in continuous squared functions:
    \[
    (x - a)^2 = x^2 -2ax - a^2 = \alpha (x^2 -2bx + b^2) + \beta (x^2 -2cx + c^2) + \gamma = \alpha (x- b)^2 + \beta (x-c)^2 + \gamma,
    \]
    for some value of $\alpha, \beta$, and $\gamma$. Therefore, in order to get a full column rank of $\bar{\Abf}$ in the equality subsystem, at most 2 rows can be selected from the first block of matrix $\Abf$. The rest $k-2$ rows need to be selected from the second block. In our column removal interpretation (see the proof of Theorem \ref{thm:ermloss-abs}), this also corresponds to restricting the number of remaining columns to at most 2.

    For each extreme point in $\Dbb$ with a single non-zero component of $\qvec$ (let us call it $i$), we can easily construct the corresponding equality by selecting $i$-th row from the first block of $\bf A$, and the remaining indices from the second block, resulting in the solution that put $\bar{q}_i = 1$ probability.
    For each extreme point in $\Dbb$ with two non-zero components of $\qvec$ (let us call it $i$ and $j$) with $q_i = \frac{ 2(j - l) + 1}{2 \left(j - i \right)}$ and $q_j = \frac{ 2(l - i) - 1}{2 \left(j - i \right)}$ where $i < l \leq j $, we construct the corresponding equality subsystem of the polytope $\Cbb$ as follows. We select all rows from the second block except $i$-th and $j$-th rows, leaving the $i$-th and $j$-th columns in our column removal interpretation. We also select $(l-1)$-th and $l$-th rows from the first block. The solution from the resulting equation subsystem is to set:
    \begin{align}
    \bar{q}_i &= \frac{  \Lbf_{(l-1,j)} -  \Lbf_{(l,j)}   }
	  { \Lbf_{(l,i)} -  \Lbf_{(l-1,i)} + \Lbf_{(l-1,j)} -  \Lbf_{(l,j)} }   \\
	  &=  \frac{  (j - l +1)^2 -  (j-l)^2   }
	  { (i-l)^2 -  (i-l+1)^2 + (j-l+1)^2 -  (j-l)^2 } =
	  \frac{ 2(j - l) + 1}{2 \left(j - i \right)}, \\
	 \bar{q}_j &= \frac{  \Lbf_{(l,i)} -  \Lbf_{(l-1,i)}    }
	  { \Lbf_{(l,i)} -  \Lbf_{(l-1,i)} + \Lbf_{(l-1,j)} -  \Lbf_{(l,j)} }   \\
	  &=  \frac{  (i - l)^2 -  (i-l+1)^2   }
	  { (i-l)^2 -  (i-l+1)^2 + (j-l+1)^2 -  (j-l)^2 } =
	  \frac{ 2(l - i) - 1}{2 \left(j - i \right)}, \\
	  \bar{v} &= \frac{ \left( \Lbf_{(j,l-1)} -  \Lbf_{(j,l)} \right) \Lbf_{(i,l)}  + 
	  \left( \Lbf_{(l,i)} -  \Lbf_{(l-1,i)} \right)  \Lbf_{(l,j)}  }
	  { \Lbf_{(l,i)} -  \Lbf_{(l-1,i)} + \Lbf_{(l-1,j)} -  \Lbf_{(l,j)} } \\
	  &=  \frac{  \left( 2(j - l) + 1 \right) (l-i)^2 + \left( 2(l - i) - 1 \right) (j-l)^2 }
	  { 2 \left(j - i \right) } .
    \end{align}
    This extreme point is the same as the one $\Dbb$ we started with.
    
    To complete our proof that $\Dbb = \Cbb$, w will show that any equality subsystem with $\rank(\bar{A}) = k+1$ in $\Cbb$ will not produce additional extreme points. Let us call the set of selected rows from the first block as $S$ and the set of remaining column indices in our column removal interpretation as $R$. There are few cases that we need to have a look:
    \begin{enumerate}%[noitemsep,topsep=0pt]
        \item The case where $S = \{i\}$ and $R = \{j\}$, but $i \neq j$. \\
        In this case, satisfying the $i$-th equality from the first block and the non-negativity constraints will make the value of $\bar{v}$ big such that the strict inequality from the $j$-th row of the first block of $\Abf$ cannot be satisfied. Therefore, the solution of the system of equation lies outside the polytope $\Cbb$.
        \item The case where $R = \{i,j\}$, and $S =\{m,l\}$ but it does not satisfy our requirement that $i \leq m < l \leq j$, and $ m = l-1$. \\
        Similar to the first case, the solution of this equation also lies  outside the polytope $\Cbb$ since satisfying the $m$-th and $l$-th equalities from the first block of $\Abf$ with the non-negative constraints will cause at least one inequality from the unselected rows of $\Abf$ cannot be satisfied due to the big value of $\bar{v}$. Hence, it is not an extreme point of $\Cbb$.
    \end{enumerate}
    
    Therefore, we show that there is no additional extreme points in $\Cbb$, and hence $\Dbb = \Cbb$, which concludes our proof.

\subsection{Proof for Theorem 11}

    The $\text{AL}^{\text{abstain}}$ above corresponds to the set of extreme points where only a single element of $\qvec$ is non zero with probability of one, or two non-zero elements of $\qvec$ are allowed 
    (let us call them $i$ and $j$) where the probability of $q_i = 1 - \alpha$ and $q_j = \alpha$ for any $i,j \in \{1,\hdots,k\}, i \neq j $ with the value of $v$ is $\alpha$. 
    Let us call the convex polytope defined by the convex hull of this set of extreme points as $\Dbb$. We need to show that $\Dbb = \Cbb$. 

    First, we show that every extreme point in $\Dbb$ is also an extreme point in $\Cbb$.
    For each extreme point in $\Dbb$ with single non-zero components of $\qvec$ (let us call it $i$), we can easily construct the corresponding equality by selecting $i$-th row from the first block of $\bf A$, and the remaining indices from the second block, resulting in the solution that put $\bar{q}_i = 1$ probability.
    For each extreme point in $\Dbb$ with two non-zero components of $\qvec$ (let us call it $i$ and $j$) with $q_i = 1 - \alpha$ and $q_j = \alpha$, we construct the corresponding equality subsystem of the polytope $\Cbb$ 
    by selecting $i$-th row and $k+1$-th row (the abstain row) from the first block, as well as
    all rows except the $i$-th and $j$-th rows from the second block. The solution from the resulting equation subsystem is to set $\bar{q}_i = 1-\alpha$,  $\bar{q}_j = \alpha$ and 0 for other indices, with the value of $\bar{v}$ equals to $\alpha$.
    This extreme point is the same as the one in $\Dbb$ we started with.
    
    Note that the extreme points we listed above corresponds to the case where only single row from the first block can be selected and the same index corresponds to the row is not selected from the second block, with an option to include the abstain row. 
    % If there are more than one regular rows are selected from the first block then:
    There are few other cases that we need to consider:
    \begin{enumerate}%[noitemsep,topsep=0pt]
        \item Two regular rows are selected from the first block where their indices are not selected from the second block and the value of $\alpha = \frac12$.\\
        In this case, the solution is to put the value of $\qvec$ corresponds to the indices of those rows to be $\frac12$, and zero to the rest. This extreme point is already in our consideration.
        \item Other cases:\\ 
        (a) two regular rows are selected from the first block and $\alpha < \frac12$, or\\
        (b) more than two regular rows are selected from the first block, or\\
        (c) the indices of one or more of the selected regular rows from the first block are also selected from the the second block. \\
        In these cases, the solution of the resulting equation lies outside the polytope $\Cbb$ since satisfying the equations of the selected rows from the first block of $\Abf$ with non zero constraints will make the value of $\bar{v}$ too big so that it cannot be satisfied by the abstain row's inequality, i.e.: $\Lbf_{(k+1,:)} \qvec - v < 0$.
    \end{enumerate}
    
    Therefore, we show that there is no additional extreme points in $\Cbb$, and hence $\Dbb = \Cbb$, which concludes our proof.

\section{Proofs for Section 4 and Section 5}

\subsection{Proof of Theorem 12}

We will analyze the optimal $\pvec$ and $v$ using the Karush Kuhn Tucker (KKT) conditions which is a necessary and sufficient optimality condition for linear program \citep{boyd2004convex}.
The Lagrangian of the minimization in Eq. \eqref{eq:lp-pred} can be written as:
\begin{align}
    \Lcal = \min_{\pvec, v} \max_{\avec \ge 0, \bvec \ge 0, c} & \;
    v - \avec^\intercal (v{\bf 1} - \Lbf^\intercal \pvec - \fvec) - \bvec^\intercal \pvec - c (\pvec^\intercal{\bf 1} - 1),
\end{align}
where $\avec, \bvec$, and $c$ are the Lagrange dual variable. The KKT condition for Eq. \eqref{eq:lp-pred} are the following:
\begin{enumerate}[noitemsep,topsep=0pt]
    \item Primal feasibility:
        $
            p_i \ge 0; \;\; \pvec^\intercal{\bf 1} = 1; \;\; v \ge \Lbf_{(:,i)}^\intercal \pvec + f_i .
        $
    \item Dual feasibility:
        $
            a_i \ge 0; \;\; b_i \ge 0.
        $
    \item Complementary slackness:
            $a_i (v - \Lbf_{(:,i)}^\intercal \pvec - f_i) = 0$, and
            $b_i p_i = 0$.
    \item Stationary:
        \begin{flalign}
            &\nabla_\pvec \Lcal = \textstyle\sum_i a_i \Lbf_{(:,i)} - \bvec - c{\bf 1}= 0 \quad \Rightarrow \quad \textstyle\sum_i a_i \Lbf_{(:,i)} - \bvec = c{\bf 1} \label{eq:pred-nabla-p}\\
            &\nabla_v \Lcal = 1 - \textstyle\sum_i a_i = 0 \quad \Rightarrow \quad \textstyle\sum_i a_i  = 1. \label{eq:pred-nabla-v}
        \end{flalign}    
\end{enumerate}

We now focus on the case where $0 \le \alpha < \frac12$.
The complementary slackness condition suggests that for non-zero elements of $\pvec$, its corresponding element in $\bvec$ must be 0. The stationary condition (Eq. \eqref{eq:pred-nabla-p}) makes sure that $\sum_i a_i \Lbf_{(:,i)} - \bvec$ is a uniform vector where all its elements are $c$.
If the element of $\pvec$ corresponds to the abstain option has non zero probability, then the value of $c$ must be $\alpha$ due to Eq. \eqref{eq:pred-nabla-v}.
Combining these conditions, it can be inferred that only at most two non-zero elements of $\pvec$ is possible for the optimal solution with one of these configurations: 
\begin{enumerate}%[noitemsep,topsep=0pt]
    \item one element of $\pvec$ corresponds to a regular class label has probability of 1, or
    \item the element of $\pvec$ corresponds to the abstain prediction has probability of 1, or
    \item two elements has non zero probability: one element corresponds to a regular class, and one element corresponds to the abstain element.
\end{enumerate}

Denote $\evec = \sum_i a_i \Lbf_{(:,i)}$, then the last row of $\evec$ (the abstain row) must be $\alpha$. A configuration of $\pvec$ with more than one non-zero probability regular classes cannot be the optimal solution. The reason is that the value of $c$ needs to be $c < \alpha < \frac12$ due to
the requirement that $b_\alpha = 0$ if the abstain option has non-zero probability, or $b_\alpha \geq 0$ if the abstain option has zero probability where $b_\alpha$ denotes the value of $\bvec$ for the abstain option. However, in the case that $\alpha < \frac12$, satisfying the conditions that $e_i = e_j$ for all $i$ and $j$ in the set of regular classes with non-zero probability requires $c \ge \frac12$.

% Denote $\evec = \sum_i a_i \Lbf_{(:,i)}$. A configuration of $\pvec$ with more than one non-zero probability regular classes and non-zero probability abstain option cannot be the optimal solution since the conditions that $e_i = e_j = \alpha$ for all $i$ and $j$ in the set of regular classes with non-zero probability cannot be satisfied. A configuration of $\pvec$ with more than one non-zero probability regular classes and zero probability abstain option cannot be the optimal solution either. The reason is that the value of $c$ needs to be $c < \alpha < \frac12$ due to the feasibility condition $b_i \geq 0$, but in the case that $\alpha < \frac12$, satisfying the conditions that $e_i = e_j$ for all $i$ and $j$ in the set of regular classes with non-zero probability requires $c \ge \frac12$.

We analyze the optimal objective for the possible optimal solutions as follows:
\begin{enumerate}%[noitemsep,topsep=0pt]
\item One element of $\pvec$ corresponds to a regular class (denoted as $p_{i^*}$)  has probability of 1.\\
In this case, $a_{i^*}$ has to be non-zero to make sure that $\sum_i a_i \Lbf_{(:,i)} - \bvec = \evec - \bvec$ is a uniform vector with value of $c$, because $b_{i^*} = 0$ due to the complementary slackness condition. The abstain row of $\evec$ implies that $c < \alpha < \frac12$, and its $i^*$-th row implies that $c = 1 - a_{i^*}$, hence  $a_{i^*}$ has to be non-zero.
Then, since $a_{i^*}$ is non zero, $v = \Lbf_{(:,i^*)}^\intercal \pvec + f_{i^*} = f_{i^*}$ has to hold. The primal feasibility of $v$ implies that that $v = f_{i^*} \geq 1 + f_{j}, \forall j \in \{1,\hdots,k\}\backslash i^*$. 
\item Two elements have non-zero probability: one element is a regular class (denoted as $p_{i^*}$), and another element is the abstain element (denoted as $p_{\alpha}$). \\
Similar to the previous case, $a_{i^*}$ has to be non zero, and $v = \alpha p_{\alpha} + f_{i^*}$ due to the complementary slackness condition. The primal feasibility of $v$ implies that that $v \geq p_{i^*} + \alpha p_{\alpha} + f_j, \forall j \in \{1,\hdots,k\}\backslash i^*$. Since there needs to be another non zero $a_j$, to satisfy the primal feasibility of $v$, the equality $v = p_{i^*} + \alpha p_{\alpha} + f_{j^*}$, where $j^* = \argmax_{j \in \{1,\hdots,k\}\backslash i^*} f_j$. This implies that $p_{i^*} = f_{i^*} - f_{j^*}$ and $p_{\alpha} =  1 - (f_{i^*} - f_{j^*})$, where $i^*$ and $j^*$ are the indices of the best and the second best potentials respectively.
\item The element of $\pvec$ corresponds to the abstain prediction has 1 probability.\\
Following the analysis in the previous item, this happens when $f_{i^*} = f_{j^*}$
\end{enumerate}

Combining the analysis above, we can conclude that for $0 \le \alpha < \frac12$, given a new datapoint $\xvec$ and its potential vector $\fvec$ where $f_i = {\theta^*}^\intercal\phi(\xvec, i)$, the optimal predictor's probability $\pvec^*$ has the following elements:
\begin{align}
    p^*_{i^*} = \begin{cases} 
      1 & f_{i*} \geq 1\!+\!f_{j^*} \\
      f_{i*}\!-\!f_{j^*} & \text{otherwise}
   \end{cases},
   \quad
   p^*_{\alpha} = \begin{cases} 
      0 & f_{i*} \geq 1\!+\!f_{j^*} \\
      1\!-\!(f_{i*}\!-\!f_{j^*}) & \text{otherwise}
   \end{cases},
   \quad
   \begin{matrix}
   p^*_l = 0, \\ \forall l \in \{1,\hdots,k\}\backslash i^*,
   \end{matrix}
\end{align}
where $i^*$ and $j^*$ are the indices of the best and the second best potentials respectively, and $p_{\alpha}$ is the probability for abstain option.
In the case that $\alpha = \frac12$, the optimal $\pvec$ is not unique (i.e. some optimal $\pvec$ can have two non zero probability of regular classes). However, using the similar technique, we can show that the $\pvec^*$ described above is one of the optimal solution.

\subsection{Proof of Theorem 14}

	Denote $\pvec$ as the probability mass given by the predictor player $\Phat(\hat{Y}|\xvec)$,
	$\qvec$ as the probability mass given by the adversary player $\Pcheck(\check{Y}|\xvec)$, and $\dvec$ as the probability mass of the true distribution $P(Y|\xvec)$.
	So, all $\pvec$, $\qvec$, and $\dvec$ lie in the $k$ dimensional probability simplex $\Delta$, where $k$ is the number of classes.
	Let $\Lbf$ be a $k$-by-$k$ loss matrix whose $(y', y)$-th entry is $\text{loss}(y', y)$.
	Let $\fvec \in \RR^{k}$ be the vector encoding of the value of $f$ at all classes.
	The definition of $f^*$ in Eq. \eqref{eq:def_consistency}   
	now becomes:
	\begin{align}
		\fvec^* &\in \argmin_\fvec \max_{\qvec \in \Delta} \min_{\pvec \in \Delta} \cbr{\fvec^\intercal \qvec + \pvec^\intercal \Lbf \qvec - \dvec^\intercal \fvec}
		\\		
		\label{eq:proof_consistency_f}
		&=\argmin_\fvec \max_{\qvec \in \Delta} \cbr{\fvec^\intercal \qvec + \min_{y'} (\Lbf \qvec)_{y'} - \dvec^\intercal \fvec}.
	\end{align}
	%So the definition of $\pi^*$ is equivalent to  
	%$\pi^* = \argmax_\pi f^*_\pi$. % and $\pi^\diamond = \argmin_\pi (C \dvec)_\pi$.
	
% 	Let us assume that $\Pi^\diamond = \argmin_\pi \mathbb{E}_{\pibar | x \sim P} [\text{loss}(\pi, \pibar)]$ (or equivalently $ \argmin_\pi (C \dvec)_\pi$) has a unique solution which we denote as $\pi^\diamond$ (we will drop this assumption later). 
	Let $\Ycal^\diamond \triangleq \argmin_{y'} \mathbb{E}_{Y | \xvec \sim P} [\text{loss}(y', Y)]$ (or equivalently $ \argmin_{y'} (\Lbf \dvec)_{y'}$) contains only a singleton
	which we denote as $y^\diamond$. 
	We are to show that $\argmax_y f^*(\xvec,y)$ is a singleton,
	and its only element $y^*$ is exactly $y^\diamond$.
	Since $\fvec^*$ is an optimal solution,
	the objective function must have a zero subgradient at $\fvec^*$.
	That means $\zero = \qvec^* - \dvec$,
	where $\qvec^*$ is an optimal solution in Eq. \eqref{eq:proof_consistency_f} under $\fvec^*$.
	As a result:
	\begin{align}
	    \label{eq:d_in_argmax}
		\dvec \in \argmax_{\qvec \in \Delta} \cbr{\qvec^\intercal \fvec^* + \min_{y'} (\Lbf\qvec)_{y'}}.
	\end{align}
	
	By the first order optimality condition of constrained convex optimization 
	(see Eq. (4.21) of \citep{boyd2004convex}),
	this means (let $\Lbf_{(y^\diamond,:)}$ be the $y^\diamond$-th row of $\Lbf$):
	\begin{align}
	\label{eq:1st_optimality}
	  \left(\fvec^* + {\Lbf_{(y^\diamond,:)}}^\intercal\right)^\intercal (\uvec - \dvec) \le 0 \quad \forall \uvec \in \Delta,
	\end{align}
	where $\fvec^* + {\Lbf_{(y^\diamond,:)}}^\intercal$ is the gradient of the objective in Eq. \eqref{eq:d_in_argmax} with respect to $\qvec$ evaluated at $\qvec = \dvec$.
	Here we used the definition of $y^\diamond$.
	However, this inequality can hold for some $\dvec \in \Delta_k \cap \RR_{++}^{k}$ 
	only if 
	$\fvec^* + {\Lbf_{(y^\diamond,:)}}^\intercal$ is a uniform vector,
	\ie, $f^*_y + \text{loss}(y^\diamond, y)$ is a constant in $y$.
	To see this, let's assume the contrary that $\vvec \triangleq \fvec^* + {\Lbf_{(y^\diamond,:)}}^\intercal$ is not a uniform vector, and let $i$ be the index of its maximum element. Let $\uvec$ be a vector whose values are 1 for index $i$ and 0 otherwise. It is clear that for any $\dvec \in \Delta_k \cap \RR_{++}^{k}$, $\vvec^\intercal \uvec > \vvec^\intercal \dvec$, and hence $\left(\fvec^* + {\Lbf_{(y^\diamond,:)}}^\intercal\right)^\intercal (\uvec - \dvec) > 0$, which does not satisfy the optimality condition.
	
	Finally, using the assumption that $\text{loss}(y, y) < \text{loss}(y', y)$ for all $y' \neq y$,
	it follows that $y^*  = y^\diamond$, since 
% 	$\argmax_y f^*(\xvec,y) = \argmin_y (\Lbf_{(y^\diamond,:)})_y$.
	$\argmax_y f^*(\xvec,y) = \argmin_y \Lbf_{(y^\diamond,y)}$.

\subsection{Proof of Theorem 15}

	Let $\Ycal^\diamond$ be the set containing all of the solution of $\argmin_{y'} (\Lbf \dvec)_{y'}$, i.e., $\Ycal^\diamond = \{ y^\diamond \mid (\Lbf \dvec)_{y^\diamond} = \min_{y'} (\Lbf \dvec)_{y'} \}$. 
	The analyses in the proof of Theorem \ref{thm:singlemin} still apply to this case, except for the Eq. \eqref{eq:1st_optimality}. Denote $h(\qvec) \triangleq \qvec^\intercal \fvec^* + \min_{y'} (\Lbf \qvec)_{y'}$. The sub-differential of $h(\qvec)$ evaluated at $\qvec = \dvec$ is the set:
	\begin{align}
	  \label{eq:subdiff}
	  \partial h(\dvec) = \{\fvec^* + \vvec \mid \vvec \in \text{\bf conv}\{{\Lbf_{(y^\diamond,:)}}^\intercal \mid y^\diamond \in \Ycal^\diamond \} \},  
	\end{align}
	where $\text{\bf conv}$ denotes the convex hull of a finite point set.
	By extending the first order optimality condition to the subgradient case, this means that there is a subgradient $\gvec \in \partial h(\dvec) $ such that:
	\begin{align}
	\label{eq:1st_optimality_subgrad}
	  \gvec^\intercal (\uvec - \dvec) \le 0 \quad \forall \uvec \in \Delta.
	\end{align}
	
	Similar to the singleton $\Ycal^\diamond$ case, this inequality can hold for some $\dvec \in \Delta \cap \RR_{++}^{k}$ 
	only if 
	$\gvec$ is a uniform vector.
	Based on Eq. \eqref{eq:subdiff}, $\gvec - \fvec^*$ can be written as a convex combination of the elements in $\Ycal^\diamond$, and thus: 
	\begin{align}
	 \fvec^* = c \one - \sum_{y' \in \Ycal^\diamond} \alpha_{y'} {\Lbf_{(y',:)}}^\intercal, \label{eq:f_star_multi}    
	\end{align}
	for some set of $\alpha_{(\cdot)} \ge 0$, $\sum_{y' \in \Ycal^\diamond} \alpha_{y'} = 1$ and some constant $c$. This means that multiple solutions of $\fvec^*$ are possible. 
	Let us denote the set of containing all solutions as $\Fcal^*$.
	For each element $y^\diamond$ in $\Ycal^\diamond$, we can recover a $f^*_{y^\diamond}$ in which the $\argmax_y f^*_{y^\diamond}(\xvec,y)$ contains a singleton element $y^\diamond$ by using Eq. \eqref{eq:f_star_multi} with  $\alpha_{y^\diamond} = 1$ and $\alpha_{y'\in \{\Ycal^\diamond\setminus y^\diamond\}} = 0$. 
	This is implied by our loss assumption that $\text{loss}(y, y) < \text{loss}(y', y)$ for all $y' \neq y$, and hence $\argmax_y f^*_{y^\diamond}(\xvec,y) = \argmin_y \Lbf_{(y^\diamond,y)}$. 
	
	Furthermore, if we add another assumption on the loss function such that it satisfies $\argmin_y \sum_{y' \in \Ycal^\diamond} \alpha_{y'} \text{loss}(y', y) \subseteq \Ycal^\diamond$ for all $\alpha_{(\cdot)} \ge 0$, $\sum_{y' \in \Ycal^\diamond} \alpha_{y'} = 1$, 
	then it follows that $\argmax_y f^*(\xvec,y) \subseteq \Ycal^\diamond$ for all $f^* \in \Fcal^*$, 
	since for any loss function that satisfy the assumption, $\argmin_y \sum_{y' \in \Ycal^\diamond} a_{y'} {\Lbf_{(y',y)}}  \subseteq \Ycal^\diamond$ for all  $\alpha_{(\cdot)} \ge 0$, $\sum_{y' \in \Ycal^\diamond} \alpha_{y'} = 1$.

\subsection{Proof of Theorem 16}

	Denote $\pvec$ as the probability mass given by the predictor player $\Phat(\hat{Y}|\xvec)$,
	$\qvec$ as the probability mass given by the adversary player $\Pcheck(\check{Y}|\xvec)$, and $\dvec$ as the probability mass of the true distribution $P(Y|\xvec)$.
	Let $\Lbf$ be a $l$-by-$k$ loss matrix whose $(y', y)$-th entry is $\text{loss}(y', y)$.
	Note that we allow the set of predictor's $l$ prediction options to be different than the number of classes $k$ in the ground truth dataset.
	Both the true probability mass and the adversary's, $\dvec$ and $\qvec$ lie in the $k$ dimensional probability simplex $\Delta^k$, wheras the predictor's probability mass lies in the $l$ dimensional probability simplex $\Delta^l$.
	Let $\fvec \in \RR^{k}$ the vector encoding of the value of $f$ at all classes.
	The potential function minimizer $f^*$ can now be written as:
	\begin{align}
		\fvec^* &\in \argmin_\fvec \max_{\qvec \in \Delta^k} \min_{\pvec \in \Delta^l} \cbr{\fvec^\intercal \qvec + \pvec^\intercal \Lbf \qvec - \dvec^\intercal \fvec}. \label{eq:proof_consistency_f2}
	\end{align}
	The Bayes optimal prediction under the loss matrix $\Lbf$ and the true distribution $\dvec$ is:
	\[
	    \argmin_{y'} (\Lbf \dvec)_{y'}.
	\]
	
	As noted in our previous analysis, since $\fvec^*$ is an optimal solution,
	the objective function must have a zero subgradient at $\fvec^*$.
	That means $\zero = \qvec^* - \dvec$, or $\qvec^* = \dvec$,
	where $\qvec^*$ is an optimal solution in Eq. \eqref{eq:proof_consistency_f2} under $\fvec^*$. Plugging back this solution to Eq. \eqref{eq:proof_consistency_f2}, and allowing the adversary player to play first, the optimal predictor's probability mass under the potential minimizer $\fvec^*$ is:
	\begin{align}
		\argmin_{\pvec \in \Delta^l} \cbr{{\fvec^*}^\intercal \dvec + \pvec^\intercal \Lbf \dvec - \dvec^\intercal \fvec^*}
		= \argmin_{\pvec \in \Delta^l} \pvec^\intercal \Lbf \dvec 
	\end{align}
	The solution of the minimization above is to put probability of 1 to the index that minimize the vector $\Lbf \dvec$ and zero to the rest, which is equal to finding a prediction that minimize $\Lbf \dvec$, i.e.: 
	\begin{align}
	    \argmin_{y'} (\Lbf \dvec)_{y'}.
	\end{align}
	This prediction is exactly equal to the Bayes optimal prediction under the loss matrix $\Lbf$ and the true distribution $\dvec$.
